# Supplementary material for: SmartInv: Multimodal Learning for Smart Contract Invariant Inference
Source: arXiv:2411.09217 source file (2024-11-14)
Supplement: Supplementary file 1 [file Appendix.tex]

\appendix
\section{Appendix}
%\subsection{Hyperparameters}\label{appendix:E}
\begin{table}[!h]

\setlength{\tabcolsep}{4pt}

\footnotesize
\caption{Hyperparameters. LR: Learning Rate. DO: Drop Out. RP: Repetitive Penalty. temp: tempature.}
\label{hyperparam}
\centering
\rowcolors{2}{white}{gray!30}
\begin{tabular}{llllll}
\toprule
Model & Epochs & LR & DO  & RP & Other \\
\midrule
LLaMA-7B  & 30 & 0.001 & 0.01  & 0.8 & Alpha=32, R=8\\
Alpaca  & 30 & 0.001 & N/A  & 0.8 & temp=0.2 \\
T5-Small  & 30 & 0.001 & N/A  & 2.0 & num\_beams=2\\
GPT2  & 30 & 0.001 & N/A  & 2.0 & N/A\\
OPT-350M  & 30 & 2e-5 & N/A  & 1.5 & N/A\\
\bottomrule
\end{tabular}
\end{table}
