# Supplementary material for: SmartInv: Multimodal Learning for Smart Contract Invariant Inference
Source: arXiv:2411.09217 source file (2024-11-14)
Supplement: Supplementary file 2 [file Appendix_A.tex]

\appendix
\section{Appendix}
\begin{table*}[!t]
\setlength{\tabcolsep}{6pt}
\footnotesize
\centering

\caption{\sys Detected Bug Classification}
\label{table:bug_description}
 \begin{tabular}{p{.15\linewidth}|p{.3\linewidth}|p{.1\linewidth}|p{.3\linewidth}}
    \toprule
      \textbf{Implementation Bugs}& \textbf{Descriptions}&\textbf{Functional Bugs} & \textbf{Descriptions}\\
     \midrule
        Reentrancy (RE) & reentering a contract repeatedly until all funds are drained; & Price manipulation (PM) &  using flashloan to manipulate price oracles;\\
     \midrule
      Integer overflow and underflow (IF) & attempting to store a value more than the maximum value allowed by a data type or attempting to store a value smaller than the minimum value allowed by a data type; & Privilege escalation (PE) & invoking privileged functions without obtaining proper access;\\  
    \midrule
     Arithmetic flaw (AF) & using incorrect mathematical formulas or incorrect computation; &Business logic flaw (BLF) & allowing arbitrary business flows unintended by developers; \\ 
     \midrule
    Suicidal contract (SC) & allowing arbitrary users to kill contracts with locked tokens in contracts; &  
     Inconsistent State update (IS) & transitioning to wrong states between transactions due to malicious execution of contracts;\\
     \midrule
     Ether leakage (EL) & leaking funds to arbitrary users due to improper access check; &Atomicity violation (AV) & violating atomicity of function executions;\\
      \midrule 
     Insufficient gas (IG) & transactions that are falsely paused due to implementations that consume high gas costs;&Cross bridge (CB) & unsafe cross-bridge funds transfer due to incorrect stateful transitions and due to the lack of domain knowledge;\\
      \midrule
    Incorrect visibility and/or ownership (IVO) & improperly setting private functions to public that allow access to unintended users or improperly allowing arbitrary users to become contract owners; & ID uniqueness violation (IDV) & violating the requirements of unique ID values intended by developers; \\    
   \bottomrule
 \end{tabular}
 \end{table*}
\subsection{RQ2: Invariants Detection Accuracy} 
\label{subsec:RQ3}
We first evaluate how accurate \sys is in generating valid invariants. We compare \sys's invariants detection capability with invariants detector \invconnq, a Daikon-adapted smart contract invariants detector, and \verismartnq, a CEGIS-style verifier. Because \sys and \invconnq\xspace generate invariants as direct output, we ran them as is. Since \verismartnq\xspace doesn't output any invariants directly, we patched up \verismartnq's\xspace intermediate invariant inference files including verifier.ml and checker.ml files to print out inferred invariants for comparable measurement. To determine ground truth of generated invariants, we first used our validation algorithm to prune model-generated invariants and manually inspected generated invariants for double checking.

\begin{comment}
\color{red} reviewer said my previous evaluation was biased, because I said the following: Neither \invconnq\xspace nor \verismartnq\xspace were able to generate invariants at the level of precise program points. Thus, we evaluated their output on more lenient standards: if their inferred invariants were correct at any given program points in the contract, we considered them as accurate. \sys inferred both invariants and associated program points of inferred invariants. Therefore, we applied stricter standards to \sys by requiring valid invariants at correct program points as an accurate output. I aim to correct the issue below \color{black}   
\end{comment}

\vspace{.1cm}\noindent\textbf{Invariants Inference Results.} Table~\ref{table:inv_table} shows the number of invariants detected by each tool. Neither \invconnq\xspace nor \verismartnq\xspace were able to generate invariants at the level of precise program points. Thus, if their inferred invariants were correct at any given program points in the contract, we considered them as accurate. \sys outperforms \invconnq\xspace and \verismartnq\xspace by 41.91\% and 64.00\% in terms of inferring valid invariants.

\vspace{.1cm}\noindent\textbf{False Positive Invariants Analysis.} Each incorrect invariant, \ie invariant that could not be validated by verifier and/or human review We examined the false positive invariants inferred by \sys. The overall pattern of false positive invariants was correct invariants with respect to contracts at large but at wrong program points. We noticed that \sys inferred correct invariants if program points were not taken into considertaion, but these invariants were associated with incorrect program points. Therefore, we did not count these invariants as accurate, because they were at incorrect program points.

In terms of the number and quality of invariants inferred,  \sys inferred (up to 10$\times$) more valid invariants than the state-of-the-arts. Table~\ref{table:inv_table} shows that \sys captured fewer but less trivial invariants compared to \invconnq\xspace. For example, \invconnq\xspace inferred invariants that were already stated in the contract source code, \eg if the source code contained \texttt{from == orig(from)}, \invconnq\xspace output \texttt{from == orig(from)} as an invariant. By comparison, \sys could reason about algebraic and loop invariants not explicitly stated in contracts. Although \verismartnq\xspace was highly effective in generating invariants against integer overflow/underflow (IF) bugs, \verismartnq\xspace could not reason about invariants that require multimodal information, such as invariants related to price manipulation. That's why \verismartnq generated fewer invariants than \sys, but produced more false positive invariants on contracts containing funcitonal bugs.

\vspace{0.1cm}\noindent\fcolorbox{black}{gray!20}{\begin{minipage}{24em}Insights from RQ2:  multimodal learning contributes positively to bug-preventive invariants generation on large contracts. The reason is that unlike existing techniques that frequently experience timeouts and errors on large contracts, foundation models do not require full contract compilation for analysis. \end{minipage}}

\subsection{RQ4: Runtime Performance}
\label{subec:runtime_performance}

 we ran each tool on the entire evaluation dataset and recorded the runtime accordingly. We also evaluated the runtime contribution of ToT's Tier 3 module by turning it on and off to measure the difference. Before presenting the results, we  first admit that our training time is amortized into inference runtime. Since \verisolnq (as is) requires manual specification, we thus approximated the manual effort of \verisolnq\xspace by consulting multiple smart contract audit companies \cite{chainlink, cypher}. We learned that each production-grade contract takes an experienced auditor from 1 hour to 3 hours. We averaged 90 minutes per contract as manual specification estimate for \verisolnq.

Table~\ref{table:runtime_table} shows the average runtime on a per contract basis. \sys outperforms static tools (\verismartnq, \verisolnq, \slithernq) by up to 125$\times$ and outperforms dynamic tools (\smartestnq, \manticorenq, \mythrilnq) by up to 163$\times$. Notably, \sys's runtime overhead does not increase by more than 30 seconds on average when the size of contract increases by 500 lines of code. As an average speedup of \sys on the entire evaluated dataset, \sys reduces overhead by up to 150$\times$. 

Since \verismartnq, \smartestnq\xspace and \manticorenq\xspace did not report runtime,  we manually measured the runtime by setting a timer when running the tools on a contract. For \mythrilnq\xspace and \slithernq\xspace, we used the tools' reported runtime.

\begin{figure}[!ht]

\centering
\includegraphics[width=0.8\linewidth]{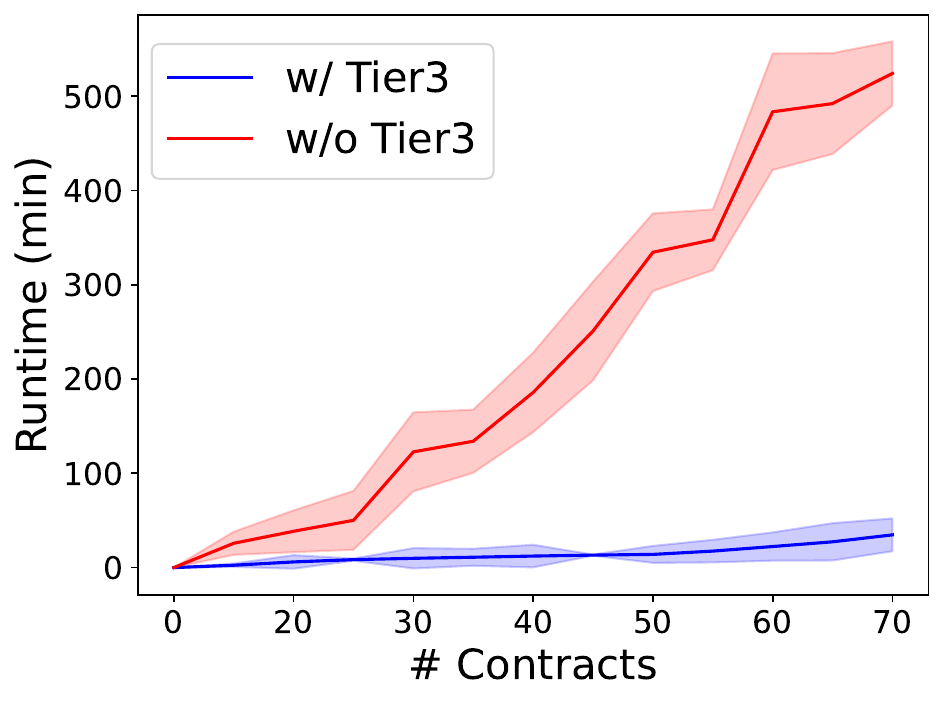}

\caption{Tier 3 runtime eval. w/ Tier3: enabling Tier3 ranking during validation. w/o Tier3: disabling Tier3 ranking during validation.}
\label{fig:algo_eval}

\end{figure}
\vspace{.1cm}\noindent\textbf{Effect of Tier 3.} Figure~\ref{fig:algo_eval} demonstrates that Tier 3 of ToT facilitated (350$\times$) faster validation runtime. We compared \sys by turning Tier 3 on and by turning it off. We noted that trivial and false positive invariants often led to timeout sessions of SAT solvers and hence failed validation in other tools. By comparison, \sys's ranking algorithm helped the validator to focus on critical and true positive invariants, and as a result, \sys found proof of (in)correctness faster.

\vspace{0.1cm}\noindent\fcolorbox{black}{gray!20}{\begin{minipage}{24em}Insights from RQ4: GPU computation along with ranked invariants provide noticeable (150x) speedup in bug detection.\end{minipage}}

\subsection{Case Study: Zero-Day Bugs}
\label{subsec:zeroday}
To illustrate \sys -detected 119 zero-day bugs, this section provides three examples and they confirmed by developers as bugs of ``high severity.'' We reported \sys' discovered zero-day bugs to developers and were reward bounty of \$17,600. We anonymized the contract in \S\ref{subsec:cross-bridge} at developers' request.

\subsection{Cross Bridge}
\label{subsec:cross-bridge}
Listing \ref{0day1} provides a buggy code snippets of a Cross Bridge contract. \sys discovers the zero-day vulnerability related to the assumed unique \texttt{\_msgHash} at line 21. Since the default value of unknown \texttt{\_msgHash} is \texttt{0x00} in solidity, this unexploited bug can potentially greenlight a malicious actor's \texttt{\_msgHash} value that defaults to \texttt{0x00} during cross bridge communication. As a result, the malicious actor can bypass the assertion check at line 21 in the public \texttt{process} function. \sys detects this vulnerability with invariant \texttt{(assert(\_msgHash) != 0)}.

% \begin{scriptsize}
\mycode
\begin{lstlisting}[float,floatplacement=H,basicstyle=\fontsize{7}{8}\selectfont, caption={Anonymized conntract code snippet}, label={0day1}, numbers=left, xleftmargin=2em]
contract Replica {
  function initialize(
    uint32 _remoteDomain,
    address _updater,
    bytes32 _committedRoot,
    uint256 _Seconds
     ) public initializer {
         __NomadBase_initialize(_updater);             remoteDomain = _remoteDomain;
        committedRoot = _committedRoot;
        //invariant #1: assert(_committedRoot != 0);
        confirmAt[_committedRoot] = 1;
        optimisticSeconds = _Seconds;
     }
...

 function process(bytes memory _message) 
    public returns (bool _success) {
    ...
    //zero day vulnerability
    @SmartInv invariant #1: assert(_msgHash != 0);
    assert(acceptableRoot(messages[_msgHash]));
    }
    
  function acceptableRoot(bytes32 _root) 
    public view returns (bool) {
    //invariant #3: assert(_root != 0);
    uint256 _time = confirmAt[_root];
     }

\end{lstlisting}
% \end{scriptsize}

\subsection{Inefficient Gas} 

Listing \ref{0day2} contains a gas inefficient \texttt{remove()} function that can lock users' funds. A user can join the vault by first joining \texttt{DepositQueue}. While on the queue, users can choose to refund their deposit or to process it at end of a transaction round. 
However, line 7 uses a gas-expensive for-loop implementation to remove each deposit on the queue. 
A long queue can easily exceed the 30 million per block gas limit even with a single deposit operation \cite{vault}. 
An attacker can send funds from different accounts to occupy the queue. 
As a result, the contract will lose the ability to refund or process users' deposits, because all deposits are locked in \texttt{DepositQueue} due to insufficient gas.

% \begin{scriptsize}
\mycode
\begin{lstlisting}[float,floatplacement=H,basicstyle=\fontsize{7}{8}\selectfont, caption={Code snippets of baseVault.sol}, label={0day2}, numbers=left, xleftmargin=2em]
abstract contract BaseVault {

    DepositQueueLib DepositQueue;

    function processQueuedDeposits(uint256 startIndex, uint256 endIndex) external {
        uint256 _totalAssets = totalAssets();
        for (uint256 i = startIndex; i < endIndex; i++){
            uint256 currentAssets = _totalAssets + processedDeposits;
            depositEntry = depositQueue.get(i);
            processedDeposits += depositEntry.amount;
        }
        @SmartInv invariant #1:
        require(depositQueue.size()==1, "Cannot process multiple deposits");
        depositQueue.remove(startIndex, endIndex);
    }
   
\end{lstlisting}
% \end{scriptsize}

\sys discovers this bug by generating an invariant after line 12 to check the size of \texttt{DepositQueue}. The inferred invariant \texttt{require(depositQueue.size() == 1,  "Cannot process multiple deposits")} ensures that there is only one deposit on the queue each time. This specified property is important for safeguarding the \texttt{remove()} function from running out of gas. 
\subsection{Arithmetic Flaws}
\label{subsec:arithmetic-bug}
\sys has detected multiple zero-day arithmetic flaw bugs. Listing \ref{0day3} shows a simplified example. This contract contains both integer overflow and arithmetic flaws. After initializing \texttt{\_stETHTransferFrom(...)}function, contract developers fail to check potential integer overflow of \texttt{amount}. \sys catches this bug by inferring an assertion invariant to properly guard the function from \texttt{amount} overflowing. This invariant ensures that the value of \texttt{amount} is always less than or equal to the maximum value that can be represented by an integer. 

At line 8, the \texttt{\_beforeWithdraw(...)} function subtracts the last share price from last round assets. However, developers fail to check the case where the subtraction might render negative \texttt{lastRoundAssets} when \texttt{sharePrice} becomes too high. \sys catches this bug by inferring an invariant that ensures that the value of \texttt{lastRoundAssets} is always non-negative. This invariant prevents the contract from executing when \texttt{lastRoundAssets} is negative.

% \begin{scriptsize}
\mycode
\begin{lstlisting}[float,floatplacement=H,basicstyle=\fontsize{7}{8}\selectfont, caption={Code snippets of StethVault.sol}, label={0day3}, numbers=left, xleftmargin=2em]
    function _stETHTransferFrom(address from, address to, uint256 amount) internal returns (...) {        
        @SmartInv invariant #1: 
        require(amount > 0);
        _asset.safeTransferFrom(from, to, amount);
      }
    }

    function _beforeWithdraw(uint256 shares) internal {
        lastRoundAssets -= shares.mulDivDown(lastSharePrice);
        @SmartInv invariant #2:
        assert(lastRoundAssets > 0);
    }
\end{lstlisting}
\subsection{Bounded Model Checking}\label{subsec.D}
We credit algorithm~\ref{algo: fullbmc} to Lahiri et al. \cite{corralalgo}.
\begin{algorithm}[!t]
\footnotesize
\setlength{\tabcolsep}{2pt}
\caption{Bounded Model Checking Procedure $BMC(S, v_i, m):$}
\label{algo: fullbmc}
\begin{tabular}{lp{2.9in}}
\textbf{Input}:
    &an input smart contract $S$, candidate invariant $v_i$, and user-specified recursion depth $m$. \\
\textbf{Input}:
    &an SMT solver $SAT$, an initial state $s_0$, a final state $s_n$. \\
\textbf{Output}:
    & Counter Example($e$) or No Counter Examples($ne$).\\
\end{tabular}
\begin{spacing}{1.1}
\begin{algorithmic}[1]
\State $P$ $\coloneqq$ \{$S$, $v_i$, assume $s_0$, $\neg{s_n}$\};
\State  $T$ $\coloneqq$ $Open\_Call\_Sites$\{$P$\};
\For{$r$ = 0 to $m$}
     \While{True}
\State     assumed value in t $\forall t \in T$ ;
\State     $SAT.Assert(\neg{t})$ \Comment{under-approximate}
     \If{$SAT.Check()$==SAT}
\State        return $e$ = $SAT.Path$;   
          \EndIf
     
 \State    $T_1$, $T_2$ = $split\_on\_recursiveDepth$ (T, i); \Comment{over-approximate}\;
\State     compute summaries $\forall t\in T_1$;
\State     assumed value $\forall t \in T_2$\;
\State    $SAT.Assert(\neg{t})$$\forall t \in T_1 \lor T_2$;
    \If{$SAT.Check()$==UNSAT $\wedge$ $T_2$ = $\emptyset$}
\State        return $ne$;
   \EndIf
     \If{$SAT.Check()$==UNSAT $\wedge$ $T_2$ $\neq$ $\emptyset$}
\State     break; 
     \EndIf
    \EndWhile
\State  $P$ $\coloneqq$  $P$ + \{$inline(t)$\};
\State  $T$ $\coloneqq$ $Open\_Call\_Sites$\{$P$\};
\EndFor
\State  return $ne$;
\end{algorithmic}
\end{spacing}
\end{algorithm}
